# Supplementary material for: Making Consistent Contacts to Graphene: Effect of Architecture and Growth Induced Defects
Source: arXiv:1601.00429 source file (2016-01-04)
Supplement: Supplementary file 1 [file supplementary-paper3.pdf]

**Contact resistance of graphene: Effect of top vs bottom contacts and growth induced defects - supplementary material**

Krishna Bharadwaj B,<sup>1</sup> Digbijoy Nath,<sup>1</sup> Rudra Pratap,<sup>1,1</sup> and Srinivasan Raghavan<sup>1,1</sup>

*Center for Nanoscience and Engineering, Indian Institute of Science, Bangalore, India*

(Dated: 17 December 2015)

## I. S1: LITERATURE SURVEY ON CONTACT RESISTIVITY OF GRAPHENE

Comparison of recent reports on the observed contact resistivity of Au contacted graphene on  $\text{SiO}_2^{1-6}$

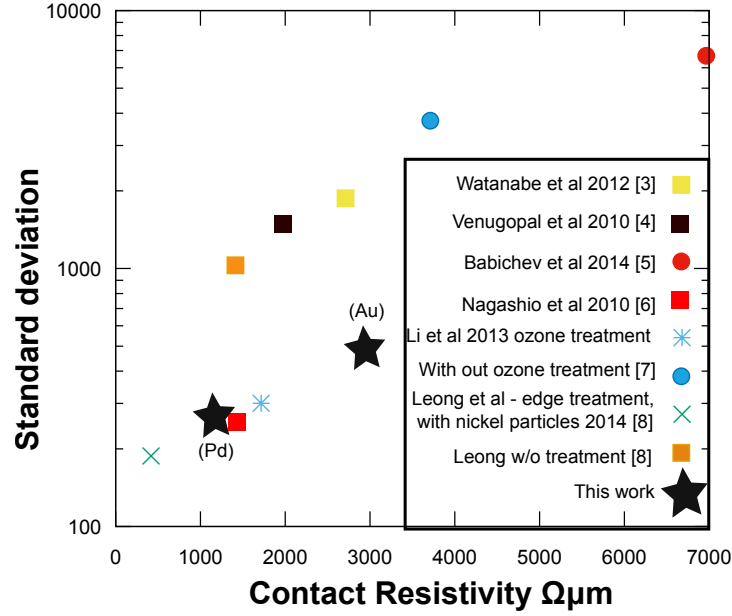

FIG. 1. Observed trends in contact resistivity and its scatter using Au as the contact metal. The results obtained in this work are also plotted for Pd and Au.

## II. S2: GRAIN SIZES OF GRAPHENE FILM

Shown Fig. S2 is a SEM image of the Cu surface, when the graphene growth has been stalled before the entire film can coalesce. The grain sizes seen here are of the order of 2-3  $\mu\text{m}$ . This suggests that the grain sizes of the graphene film after coalescence has to greater than 3  $\mu\text{m}$ .

## III. CVD GROWTH OF GRAPHENE

Graphene was grown on top of Cu foils using an in-house build CVD reactor though a process first reported by Ruoff et al.[18] 99.997 % pure methane and 99.9998 % pure

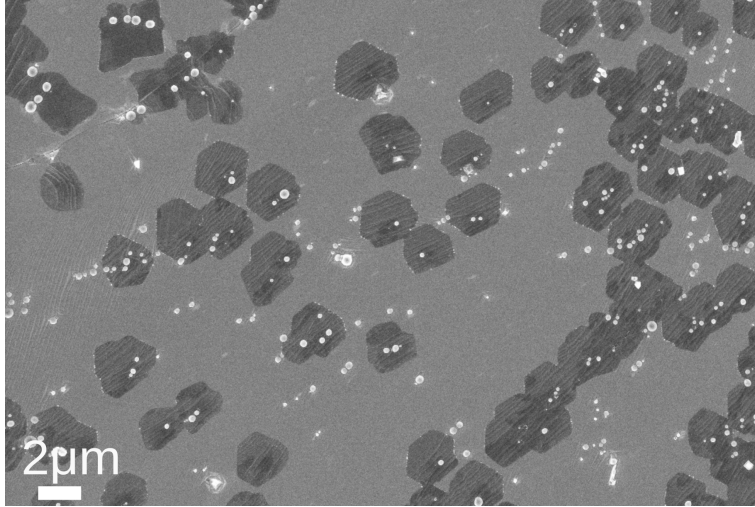

FIG. 2. Graphene grain sizes. Shown in the image is a snapshot of a partially terminated (before coalescence) graphene growth. Grains of sizes in the order of 2 - 3  $\mu\text{m}$  is seen.

hydrogen sources were used. The Cu foil was heated to 1000  $^{\circ}\text{C}$  under a hydrogen pressure of 400 Torr and annealed at the same temperature for 2 hours before all growth runs. As reported by Tsen et al.<sup>7</sup>, the methane gas flow rates determine the graphene grain size and hence the total grain boundary length per unit area in the film. This subsequently fixes the total defect density in the film as grain boundaries are the most prominent defect structures in CVD grown graphene<sup>8</sup>. Graphene growth in this letter was done using two different  $\text{CH}_4$  flow rates. Graphene with the lesser defect density was grown under 100 sccm hydrogen and 3 sccm Methane, and the graphene with the higher defect density was grown under 100 sccm  $\text{H}_2$  and 100 sccm  $\text{CH}_4$ . The lower limits on the  $\text{CH}_4$  flow was set by kinetics as the nucleation and growth rates are exceeding slow below these values<sup>9</sup>.

#### IV. DETAILS ON THE FEATURE SIZES

Due to the polycrystalline nature of the graphene film, devices of dimension smaller than 5  $\mu\text{m}$  had huge variation due to largely varying statistical distribution of the grain boundaries. Dimensions of the order of 25  $\mu\text{m}$  were chosen in this letter so that the number of boundaries in each segment of the TLM structure has a similar statistical distribution leading to consistent measurements.

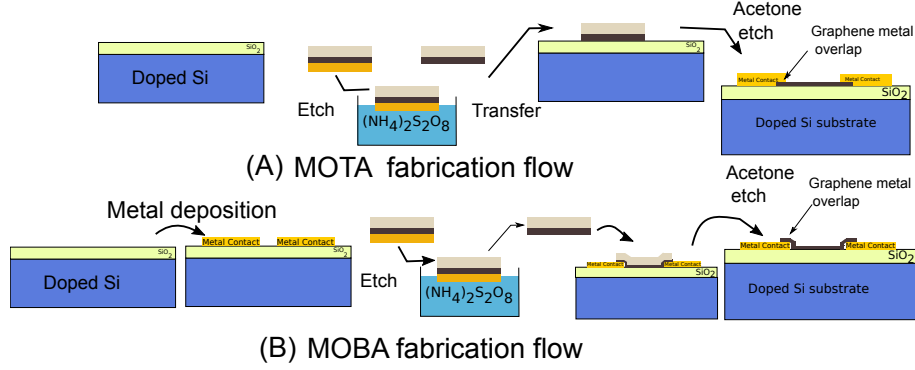

FIG. 3. MOTA vs. MOBA. (A) Top row describes the conventional MOTA fabrication flow and the bottom row describes the MOBA fabrication flow as used in this letter. The wet etch and transfer process of CVD grown graphene is common to both processes and is similar to ones described elsewhere<sup>10</sup>. While in the MOBA process graphene is transferred last, in the MOTA process, graphene is transferred prior to metal deposition steps leading to chances of trapped photo-resist residues at the metal-graphene interface.

## V. DETAILS ON FABRICATION

In both architectures, a heavily doped P-type Si wafer is used. The wafer is thermally oxidized to obtain a 300 nm thick oxide layer. In MOTA, CVD grown graphene is first transferred using the transfer process described in the main text. Once transferred, the graphene channel was defined using UV lithographic processes. A photo resist mask was obtained after selective exposure and development. Using the photo resist mask, the graphene was removed from other areas using a mild oxygen plasma. Subsequently, UV lithography was performed to open masks for metal deposition. The required metal was then deposited using E-beam evaporation. The contact pads were finally realized using lift-off in PG remover.

In MOBA, before graphene is transferred, metal contact pads were realized as described before using UV lithography and lift-off procedures. The metal surface was cleaned using a mild oxygen plasma to remove any contaminants. Subsequently, graphene is transferred onto this pre-patterned substrate as described in the main text. Finally, the channel is realized using a last lithographic step and oxygen plasma etch as described in the previous paragraph. It is to be noted here that, in MOBA, graphene contacts the metal surface which has never been in contact with photo resists or polymers, which are the usual contaminants in the device fabrication steps.

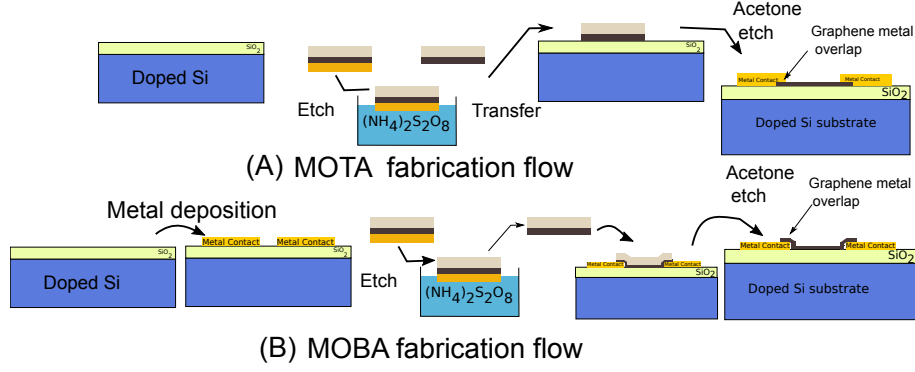

FIG. 4. MOTA vs. MOBA. (A) Top row describes the conventional MOTA fabrication flow and the bottom row describes the MOBA fabrication flow as used in this letter. The wet etch and transfer process of CVD grown graphene is common to both processes and is similar to ones described elsewhere<sup>10</sup>. While in the MOBA process graphene is transferred last, in the MOTA process, graphene is transferred prior to metal deposition steps leading to chances of trapped photo-resist residues at the metal-graphene interface.

For both MOTA and MOBA fabrication process, the AZ 5214E photo resist was spin coated on dehydrated substrates at 4000 RPM. The samples were hot plate baked at 120 °C for 1 minute. A dosage of 35 uJ/cm<sup>2</sup> was used in the EVG double sided mask aligner. Post exposure development was done using AZ 351B developer for 18 seconds to produce the required under-cut. Post lithography, the samples were either sputtered (in the case of MOBA) or thermally evaporated (in the case of MOTA). Post metallization, the lift-off was performed using the MicroChem made PG remover.

## VI. MOBILITY EXTRACTION

A representative transfer characteristics and the fitted curve is presented in the Fig. 4. The mobility is extracted from a constant mobility expression given in Eq. 2.

## VII. ELECTRICAL CHARACTERIZATION

Transfer characteristics of devices in the TLM structure are plotted together to notice the shift in the CNP. Shorter devices had smaller positive CNPs.

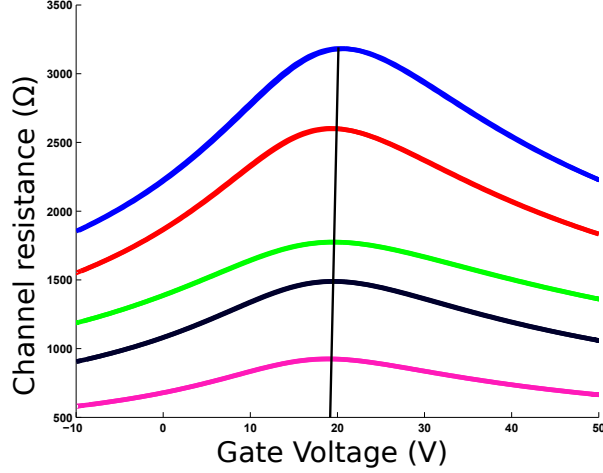

FIG. 5. Typical transfer characteristics of devices in the TLM structure. All devices have a P-type nature with CNP at positive gate voltages. The CNPs of individual devices in the TLM drift towards the zero gate voltage size as the device length shrinks.

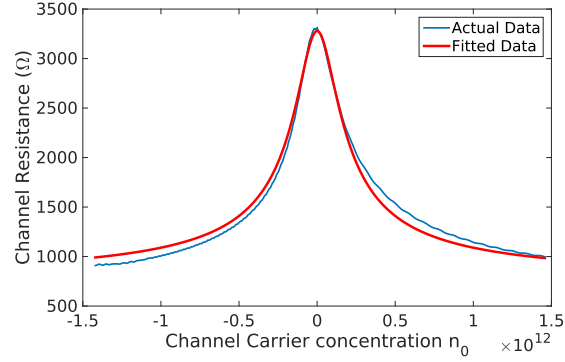

FIG. 6. A representative transfer characteristics is shown along with a fit curve using the constant mobility model. The mobility and intrinsic carrier density were extracted from the fit.

## VIII. EQUIPMENT USED

Optical Lithography was performed using a 350 nm EVG double sided mask aligner. Shipley made AZ 5214E photo resist was used. The after-exposed substrate was developed using AZ 351B developer. All the metals were sputtered for MOBA architecture and thermally evaporated for MOTA. The cumulative thickness of the adhesive layer and the contact metal was set at 80 nm in all cases.

The electrical characterization was performed using Lakeshore low pressure work station

and Agilent semiconductor impedance analyzer. The samples were current annealed at a density of  $3 \times 10^8$  A/cm<sup>2</sup> for 3 minutes and let to cool down for 5 minutes before the measurements were made. The measurements were made at a pressure of 5E-6 mbar. The Raman measurements were done using a 532 nm laser source on a Horiba made microspectrometer. All mathematical analysis and fitting was done using Matlab 8.2.

## REFERENCES

- <sup>1</sup>Eiichiro Watanabe, Arolyn Conwill, Daiju Tsuya, and Yasuo Koide. Low contact resistance metals for graphene based devices. *Diamond and Related Materials*, 24(0):171 – 174, 2012. ISSN 0925-9635. doi:<http://dx.doi.org/10.1016/j.diamond.2012.01.019>. URL <http://www.sciencedirect.com/science/article/pii/S0925963512000295>.
- <sup>2</sup>A Venugopal, L Colombo, and EM Vogel. Contact resistance in few and multilayer graphene devices. *Applied Physics Letters*, 96(1):013512, 2010.
- <sup>3</sup>AV Babichev, VE Gasumyants, A Yu Egorov, S Vitusevich, and M Tchernycheva. Contact properties to cvd-graphene on gaas substrates for optoelectronic applications. *Nanotechnology*, 25(33):335707, 2014.
- <sup>4</sup>K Nagashio, T Nishimura, K Kita, and A Toriumi. Contact resistivity and current flow path at metal/graphene contact. *Applied Physics Letters*, 97(14):143514, 2010.
- <sup>5</sup>Wei Li, Yiran Liang, Dangmin Yu, Lianmao Peng, Kurt P Pernstich, Tian Shen, AR Hight Walker, Guangjun Cheng, Christina A Hacker, Curt A Richter, et al. Ultraviolet/ozone treatment to reduce metal-graphene contact resistance. *Applied Physics Letters*, 102(18):183110, 2013.
- <sup>6</sup>Wei Sun Leong, Hao Gong, and John T. L. Thong. Low-contact-resistance graphene devices with nickel-etched-graphene contacts. *ACS Nano*, 8(1):994–1001, 2014. doi:10.1021/nn405834b. URL <http://dx.doi.org/10.1021/nn405834b>. PMID: 24328346.
- <sup>7</sup>Adam W. Tsen, Lola Brown, Mark P. Levendorf, Fereshte Ghahari, Pinshane Y. Huang, Robin W. Havener, Carlos S. Ruiz-Vargas, David A. Muller, Philip Kim, and Jiwoong Park. Tailoring electrical transport across grain boundaries in polycrystalline graphene. *Science*, 336(6085):1143–1146, 2012. doi:10.1126/science.1218948.
- <sup>8</sup>Florian Banhart, Jani Kotakoski, and Arkady V Krasheninnikov. Structural defects in graphene. *ACS nano*, 5(1):26–41, 2010. URL <http://pubs.acs.org/doi/abs/10.1021/>

nn102598m.

- <sup>9</sup>Priyadarshini Ghosh, Shishir Kumar, Gopalakrishnan Ramalingam, Vidya Kochat, Madhavan Radhakrishnan, Sukanya Dhar, Satyam Suwas, Arindam Ghosh, Narayanan Ravishankar, and Srinivasan Raghavan. Insights on defect-mediated heterogeneous nucleation of graphene on copper. *The Journal of Physical Chemistry C*, 119(5):2513–2522, 2015.
- <sup>10</sup>Xuesong Li, Weiwei Cai, Jinho An, Seyoung Kim, Junghyo Nah, Dongxing Yang, Richard Piner, Aruna Velamakanni, Inhwa Jung, Emanuel Tutuc, Sanjay K. Banerjee, Luigi Colombo, and Rodney S. Ruoff. Large-area synthesis of high-quality and uniform graphene films on copper foils. *Science*, 324(5932):1312–1314, 2009. doi:10.1126/science.1171245.
