# Supplementary material for: Making Consistent Contacts to Graphene: Effect of Architecture and Growth Induced Defects
Source: arXiv:1601.00429 source file (2016-01-04)
Supplement: Supplementary file 2 [file supplementarty.pdf]

# Supplementary materials

Comparison of recent reports on the observed contact resistivity of Au contacted graphene on SiO<sub>2</sub>

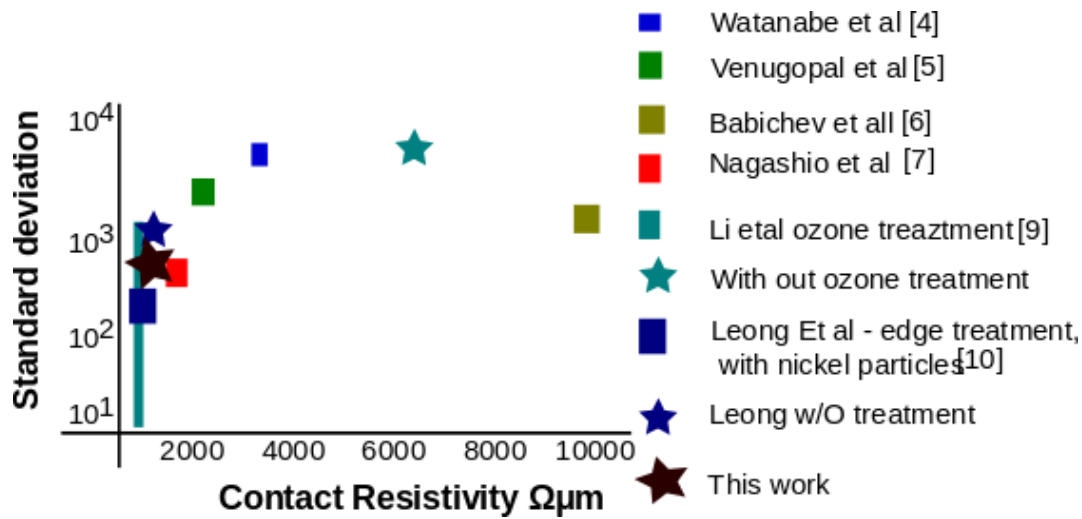

Figure S1: Observed trends in contact resistivity and its scatter. Reported contact resistivity values obtained on Au contacted graphene devices are compared against the standard deviation obtained. The values obtained in this work is also plotted for benchmarking purposes.

Grain sizes of graphene film

Shown below is a SEM image of the Cu surface, when the graphene growth has been stalled before the entire film can coalesce. The grain sizes seen here are atleast 2-3  $\mu\text{m}$ . This suggests that the grain sizes of the graphene film after coalescence has to be greater than 3  $\mu\text{m}$ .

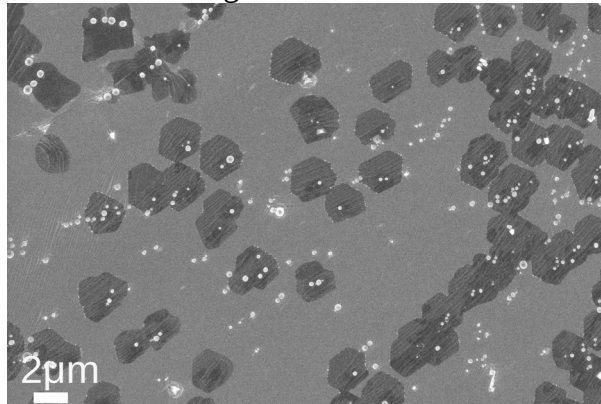

Details on Fabrication

Optical Lithography was performed using a 350 nm EVG double sided mask aligner. Shipley made AZ 5214E photo resist was used. The after-exposed substrate was developed using AZ 351B developer. All the metals were sputtered for MOBA architecture and thermally evaporated for MOTA. The cumulative thickness of the adhesive layer and the contact metal was set at 80 nm in all cases.

The electrical characterization was performed using lakeshore lop pressure work station and agilent semiconductor impedance analyzer. The samples were current annealed at a density of  $3 \times 10^8$  A/cm<sup>2</sup> for 3 minutes and let to cool down for 5 minutes before the measurements were made. The

measurements were made at a pressure of  $5 \times 10^{-6}$  mBar. The Raman measurements were done using a 532 nm laser source on a Horiba made microspectrometer. All the mathematical analysis and fitting were done using Matlab 8.2.
